# Supplementary material for: Uncertainty Quantification and Flow Dynamics in Rotating Detonation Engines
Source: arXiv:2505.02378 source file (2025-05-13)
Supplement: Supplementary file 1 [file 8_appendix.tex]

\section{Appendix}
